# Supplementary material for: Classifier Language Models: Unifying Sparse Finetuning and Adaptive Tokenization for Specialized Classification Tasks
Source: arXiv:2508.08635 source file (2025-08-12)
Supplement: Supplementary file 1 [file results.tex]

\section{Prototyping Qualitative Analysis}
\label{appendix:retrieval}

In this section, we show some qualitative examples of the prototypes from our approach.~\Cref{tab:retrieval_example_speed,tab:retrieval_example_volume,tab:retrieval_example_circuitousness} include the input as well as the retrieved sample and the generated text. In many cases, we observe that the retrieved example demonstrates a strong change in feature, and \textsc{Cev-LM} corrects the strength of the change to ensure it is closer to the target delta.

  \begin{table}[htb]
  \small
  \centering
  \caption{Examples of an input, retrieved, and edited sentence for the model trained for a change in $\textbf{speed}$ with a target delta of $0.5$.  We use a tolerance $\epsilon = 0.1$ for our approach, as it empirically provided the best results in~\Cref{subsec:tolerance}. The models are fed the input (\ie \textbf{Original}) and generate by applying an ``edit vector'' to the latent representation of the input sentence.}
  \label{tab:retrieval_example_speed} 
  \begin{tabularx}{\linewidth}{@{}>{\raggedright\arraybackslash}X@{}}
   \toprule[1.5pt]
  \textsc{Retrieved} \& \textsc{Generated Text} - \textbf{\textsc{Speed}}\\
  \midrule[0.75pt]
  \textsc{Example 1:}\\
  \textbf{Input}: I will not return, terrible customer service. \\
  \textbf{Prototype}: Poorest customer service skills. \\
  \textbf{\textsc{Cev-LM}}: Terrible , terrible customer service. \\
  \addlinespace[0.5em]
  \textsc{Example 2:}\\
  \textbf{Input}: The food in the restaurant can be a little pricey, but it's good and you get a lot of it.  \\
  \textbf{Prototype}:  The food in the restaurant is a bit pricey, but it's good. \\
  \textbf{\textsc{Cev-LM}}: The food is good, but it's pricey. \\
  \bottomrule[1.5pt]\\
  \end{tabularx}
  \vspace{-10px}
  \end{table}

  \begin{table}[htb]
  \small
  \centering
  \caption{Examples of an input, retrieved, and edited sentence for the model trained for a change in $\textbf{volume}$ with a target delta of $0.5$.  We use a tolerance $\epsilon = 0.1$ for our approach, as it empirically provided the best results in~\Cref{subsec:tolerance}. The models are fed the input (\ie \textbf{Original}) and generate by applying an ``edit vector'' to the latent representation of the input sentence.}
  \label{tab:retrieval_example_volume} 
  \begin{tabularx}{\linewidth}{@{}>{\raggedright\arraybackslash}X@{}}
   \toprule[1.5pt]
  \textsc{Retrieved} \& \textsc{Generated Text} - \textbf{\textsc{Volume}}\\
  \midrule[0.75pt]
  \textsc{Example 1:}\\
  \textbf{Input}: Overall, this was a positive experience.  \\
  \textbf{Prototype}: Overall, we had a positive experience and the food was good. \\
  \textbf{\textsc{Cev-LM}}: Overall, a very positive experience - I'll definitely be back. \\
  \addlinespace[0.5em]
  \textsc{Example 2:}\\
  \textbf{Input}: The menu had lots of options. \\
  \textbf{Prototype}: The menu leaves you with lots of options that you can customize. \\
  \textbf{\textsc{Cev-LM}}: The menu here has lots of options that we want to try. \\
  \bottomrule[1.5pt]\\
  \end{tabularx}
  \vspace{-10px}
  \end{table}

    \begin{table}[htb]
  \small
  \centering
  \caption{Examples of an input, retrieved, and edited sentence for the model trained for a change in $\textbf{circuitousness}$ with a target delta of $0.5$.  We use a tolerance $\epsilon = 0.1$ for our approach, as it empirically provided the best results in~\Cref{subsec:tolerance}. The models are fed the input (\ie \textbf{Original}) and generate by applying an ``edit vector'' to the latent representation of the input sentence.}
  \label{tab:retrieval_example_circuitousness} 
  \begin{tabularx}{\linewidth}{@{}>{\raggedright\arraybackslash}X@{}}
   \toprule[1.5pt]
  \textsc{Retrieved} \& \textsc{Generated Text} - \textbf{\textsc{Circuitousness}}\\
  \midrule[0.75pt]
  \textsc{Example 1:}\\
  \textbf{Input}: This is my favorite Szechuan restaurant in town. \\
  \textbf{Prototype}:  This is my favorite Szechuan restaurant, and probably my favorite Szechuan restaurant ever.  \\
  \textbf{\textsc{Cev-LM}}: This is my favorite Szechuan restaurant in town and probably in the world.\\
  \addlinespace[0.5em]
  \textsc{Example 2:}\\
  \textbf{Input}: The menu has a little bit of everything.  \\
  \textbf{Prototype}: The menu has a little bit of everything that you could want. \\
  \textbf{\textsc{Cev-LM}}: The menu has a little bit of this and a little bit of that. \\
  \bottomrule[1.5pt]\\
  \end{tabularx}
  \vspace{-10px}
  \end{table}

\section{Similarity Scores on Toxicity \& Formality}
\label{appendix:sim_other}

In this section, we present the similarity scores of the baseline approach and our approach over formality and toxicity as control attributes in~\Cref{tab:other_bleu_bert}. We find that the scores demonstrate our generations stay on topic, further indicating the robustness of our approach on more standard control attributes.

\begin{table*}[h]
\centering
\tiny
\caption{BLEU and BERT (F1) Scores for speed, volume, and circuitousness across all approaches for different target deltas. The scores are averaged across three training runs (inference runs for GPT-3). We use a tolerance $\epsilon = 0.1$ for all of our approaches, as it empirically provided the best results in~\Cref{subsec:tolerance}.\vspace{-5pt}}
%\footnotesize
\noindent\setlength\tabcolsep{2.9pt}
\fontsize{4pt}{4pt}\selectfont
\resizebox{\textwidth}{!}{%
\begin{tabular}{@{}p{0.20\linewidth}@{\hspace{2pt}}
% K{\newfactor\linewidth}K{\newfactor\linewidth}K{\newfactor\linewidth}@{\hspace{5pt}}
% K{\newfactor\linewidth}K{\newfactor\linewidth}K{\newfactor\linewidth}@{\hspace{5pt}}
% % K{\newfactor\linewidth}K{\newfactor\linewidth}K{\newfactor\linewidth}@{\hspace{5pt}}
% K{\newfactor\linewidth}K{\newfactor\linewidth}K{\newfactor\linewidth}@{}} \\
ccc@{\hspace{5pt}}ccc@{\hspace{5pt}}ccc@{}}
\toprule
\textbf{Metric} & \multicolumn{3}{c}{\textbf{Toxicity}}  & \multicolumn{3}{c}{\textbf{Formality}}\\
\cmidrule{2-4} \cmidrule(lr){5-7}
%\midrule
{\textbf{Target Delta}} & \textbf{0.1} & \textbf{0.5} & \textbf{0.9} & \textbf{0.1} & \textbf{0.5} & \textbf{0.9} \\

\midrule
\multicolumn{7}{c}{\textsc{\textbf{BERTScore} - Benchmark Approaches}} \\
\midrule[0pt]

\textbf{GPT-3}~\cite{brown2020language}       & 0.857 & 0.869    & 0.866 & 0.851 & 0.851  & 0.862  \\
\textbf{MuCoCO}~\cite{kumar2021controlled}    & 0.763 & 0.771    & 0.774 & 0.763 & 0.759  & 0.760  \\
\textbf{SSD-LM}~\cite{han2022ssd}             & 0.769 & 0.767    & 0.769 & 0.763 & 0.760  & 0.747 \\
\textbf{Prefix Tuning}~\cite{li2021prefix}    & 0.833 & 0.827    & 0.823 & 0.843 & 0.836  & 0.834  \\ 

\midrule[0pt]
\multicolumn{7}{c}{\textsc{\textbf{BERTScore} - Our Approaches}} \\
\midrule[0pt]

\textbf{\textsc{Cev-LM}}                      & 0.848 & 0.827    & 0.837 & 0.842 & 0.842  & 0.845   \\

\midrule
\multicolumn{7}{c}{\textsc{\textbf{BLEU} - Benchmark Approaches}} \\
\midrule[0pt]

\textbf{GPT-3}~\cite{brown2020language}       & 0.231 & 0.250    & 0.291 & 0.219 & 0.273     & 0.269 \\
\textbf{MuCoCO}~\cite{kumar2021controlled}    & 0.305 & 0.268    & 0.293 & 0.257 & 0.276     & 0.219 \\
\textbf{SSD-LM}~\cite{han2022ssd}             & 0.294 & 0.343    & 0.346 & 0.314 & 0.325     & 0.326   \\
\textbf{Prefix Tuning}~\cite{li2021prefix}    & 0.246 & 0.269    & 0.275 & 0.231 & 0.217     & 0.194 \\

\midrule[0pt]
\multicolumn{7}{c}{\textsc{\textbf{BLEU} - Our Approaches}} \\
\midrule[0pt]

\textbf{\textsc{Cev-LM}}                      & 0.320 & 0.316    & 0.295 & 0.342 & 0.334     & 0.265 \\

\bottomrule
\end{tabular}}
\label{tab:other_bleu_bert}
% \vspace{-10pt}
\end{table*}

% \begin{table}[]
% \begin{tabular}{lcccccc}
% \hline
% BERTScore     &       & Toxicity &       &       & Formality &        \\
% Target Delta  & 0.1   & 0.5      & 0.9   & 0.1   & 0.5    & 0.9    \\ \hline
% GPT-3         & 85.65 & 86.89    & 86.58 & 85.08 & 85.12  & 86.20  \\
% MuCoCO        & 76.31 & 77.08    & 77.41 & 76.31 & 75.92  & 76.01  \\
% SSD-LM        & 76.86 & 76.66    & 76.87 & 76.27 & 75.96  & 0.7472 \\
% Prefix Tuning & 83.21 & 82.73    & 82.27 & 84.34 & 83.60  & 83.39  \\ \hline
% CEV-LM        & 84.81 & 82.70    & 83.69 & 84.18 & 84.19  & 84.47 
% \end{tabular}
% \end{table}

% \begin{table}[]
% \begin{tabular}{lcccccc}
% \hline
% BLEU          &       & Toxicity &       &       & Formality &       \\
% Target Delta  & 0.1   & 0.5      & 0.9   & 0.1   & 0.5       & 0.9   \\ \hline
% GPT-3         & 0.231 & 0.250    & 0.291 & 0.219 & 0.273     & 0.269 \\
% MuCoCO        & 0.305 & 0.268    & 0.293 & 0.257 & 0.276     & 0.219 \\
% SSD-LM        & 0.294 & 0.343    & 0.346 & 0.314 & 0.325     & 0.326 \\
% Prefix Tuning & 0.246 & 0.269    & 0.275 & 0.231 & 0.217     & 0.194 \\ \hline
% CEV-LM        & 0.320 & 0.316    & 0.295 & 0.342 & 0.334     & 0.265
% \end{tabular}
% \end{table}

\section{Tolerance Tuning}
\label{appendix:tolerance}

\begin{table*}[]
  \centering
  \small
  \caption{Evaluation metrics (BLEU \cite{Papineni2002bleu} and BERTScore \cite{zhang2019bertscore}) and strength of control on $\Delta$ for the trained models (ideally, $\Delta = 0.5$) for speed. The scores are averaged across three training runs with different seeds. We train a baseline edit-then-prototype model \cite{guu2018generating}, as well as \textsc{Cev-LM ($\mathcal{N}$-only)} and \textsc{Cev-LM} with different tolerances ($\epsilon$). We record both train and test BLEU to demonstrate overfitting with lower tolerances. }
  \label{tab:eval-tol}
  \begin{tabularx}{0.9\linewidth}{@{}>{\raggedright\arraybackslash}Xcccc@{}}
   \toprule[1.5pt]
  \textsc{Model} & \textsc{Delta} & \textsc{Train BLEU} & \textsc{Test BLEU} & \textsc{BERTScore} \\     
  \midrule[0.75pt]
  % \addlinespace[0.5em]
\textsc{Edit-then-Prototype}    & 0.0113 & \textbf{0.6691}     & \textbf{0.5679}    & 0.9327 \\
  \midrule[0.75pt]
\textsc{Cev-LM ($\mathcal{N}$-only)}: $\epsilon$ = 0.05 & 0.4559 & 0.8057     & 0.4266    & 0.9326 \\
\textsc{Cev-LM ($\mathcal{N}$-only)}: $\epsilon$ = 0.1  & 0.4558 & 0.7146     & \textbf{0.5747}    & 0.9340 \\
\textsc{Cev-LM ($\mathcal{N}$-only)}: $\epsilon$ = 0.2  & 0.4405 & 0.5994     & 0.5628    & 0.9355 \\
  \midrule[0.75pt]
% Perturbation            & 0.4433 & 0.5513     & 0.4531    & 0.9346 \\
\textsc{Cev-LM}: $\epsilon$ = 0.05  & 0.4279 & 0.5709     & 0.5218    & 0.9329 \\
\textsc{Cev-LM}: $\epsilon$ = 0.1   & 0.4455 & 0.6375     & 0.5400    & 0.9386 \\
\textsc{Cev-LM}: $\epsilon$ = 0.2   & \textbf{0.4596} & \textbf{0.6751}     & \textbf{0.5679}    & 0.9334 \\
  \bottomrule[1.5pt]\\
  \end{tabularx}
  \vspace{-10pt}
  \end{table*}

We measure the impact of $\epsilon$ on training in~\Cref{tab:eval-tol}. Too low of a tolerance value leads to overfitting, indicated by a closer $\Delta$ to the target and poor performance in the test-time similarity metrics. As mentioned before, controlled edit vector perturbations to edit vectors improves similarity metrics at the cost of $\Delta$, which implies that the approach helps to combat overfitting. At $\epsilon = 0.05$ and $\epsilon = 0.1$, we see that perturbation is generally not helpful, but at tolerance $\epsilon = 0.2$, the perturbation approach leads to a higher $\Delta$. Note that the BLEU scores are slightly different as n-grams are weighted differently in the code for the edit-then-prototype architecture \cite{guu2018generating} and in NLTK \cite{bird-loper-2004-nltk}.

\section{Controlled Edit Vector Perturbation}
\label{appendix:perturb}

In~\Cref{tab:eval}, we present the results of the neighborhood creation and neighborhood creation + perturbation approaches. The Baseline shows the out-of-the-box edit-then-prototype model, which has little impact on the target attribute and provides a rough baseline of the similarity metrics. Again, we find that as the target delta increases, the MAE increases and similarity scores decrease. This phenomenon is attributed to the data distribution and is expanded on in~\Cref{subsec:data_dist}. We observe that perturbation is sometimes helpful in decreasing MAE, especially in the case of volume. However, this behavior is inconsistent across speed and circuitousness and warrants further exploration. 

  \begin{table*}[]
  \centering
  \caption{Evaluation metrics (BLEU \cite{Papineni2002bleu} and BERTScore \cite{zhang2019bertscore}) and strength of control on $\Delta$ for the trained models. The scores are averaged across three training runs, and we omit variance due to negligible values. We train a baseline model \cite{guu2018generating} (Baseline) and multiple models across various target deltas for all nonstandard control conditions (\eg speed, volume, circuitousness) to show training has a significant impact on the achieved control.}
  \label{tab:eval}
\scalebox{0.7}{
\begin{tabularx}{1.36\linewidth}{cccccc|ccccc}

                & \multicolumn{5}{c}{\textbf{\textsc{Cev-LM ($\mathcal{N}$-only)}}} & \multicolumn{5}{c}{\textbf{\textsc{Cev-LM}}}\\
                \toprule[1.5pt]
               & \textsc{Target Delta} & \textsc{Delta} & \textsc{MAE} & \textsc{BLEU} & \textsc{BERT-F1} & \textsc{Target Delta} & \textsc{Delta} & \textsc{MAE} & \textsc{BLEU} & \textsc{BERT-F1} \\
\midrule[0.75pt]
               & Baseline  & 0.0468  & -      & 0.3185 & 0.9327 & Baseline  & 0.0468  & -      & 0.3185 & 0.9327 \\
               & 0.125     & 0.1105  & 0.0145 & 0.3399 & 0.9351 & 0.125     & 0.1189  & 0.0061 & 0.3261 & 0.9350 \\
Speed          & 0.5       & 0.4558  & 0.0442 & 0.3276 & 0.9340 & 0.5       & 0.4355  & 0.0645 & 0.3123 & 0.9386 \\
               & 2.0       & 1.7594  & 0.2406 & 0.3051 & 0.9291 & 2.0       & 1.7897  & 0.2103 & 0.2944 & 0.9281 \\
               & 4.0       & 3.6213  & 0.3787 & 0.2463 & 0.9188 & 4.0       & 3.4657  & 0.5343 & 0.2736 & 0.9230 \\
\midrule[0.75pt]
               & Baseline  & 0.0011  & -      & 0.3185 & 0.9327 & Baseline  & 0.0011  & -      & 0.3185 & 0.9327 \\
Volume         & 0.125     & 0.1106  & 0.012  & 0.3296 & 0.9380 & 0.125     & 0.1130  & 0.012  & 0.3038 & 0.9351 \\
               & 0.5       & 0.4415  & 0.0585 & 0.2682 & 0.9320 & 0.5       & 0.4535  & 0.0465 & 0.2653 & 0.9314 \\
               & 2.0       & 1.7521  & 0.2479 & 0.2869 & 0.9244 & 2.0       & 1.8466  & 0.1534 & 0.2518 & 0.9208 \\
\midrule[0.75pt]
               & Baseline  & -0.0022 & -      & 0.3185 & 0.9327 & Baseline  & -0.0022 & -      & 0.3185 & 0.9327 \\
Circuitousness & 0.125     & 0.0723  & 0.0527 & 0.2483 & 0.9271 & 0.125     & 0.0664  & 0.0586 & 0.2902 & 0.9306 \\
               & 0.5       & 0.4217  & 0.0783 & 0.2680 & 0.9109 & 0.5       & 0.4207  & 0.0793 & 0.2755 & 0.9089  \\
               & 1.0       & 0.7893  & 0.2107 & 0.2479 & 0.9082 & 1.0       & 1.0519  & 0.0519 & 0.1622 & 0.8354  \\
\bottomrule[1.5pt]\\ \\
% \midrule[0.75pt] \\
\end{tabularx}
}
\end{table*}
