# Supplementary material for: Classifier Language Models: Unifying Sparse Finetuning and Adaptive Tokenization for Specialized Classification Tasks
Source: arXiv:2508.08635 source file (2025-08-12)
Supplement: Supplementary file 3 [file model_details.tex]

\section{Hyperparameters and Other Details}
\label{appendix:hyperparams}

In this section, we provide further information about the tokenization and finetuning of our models on each test dataset.
