# Supplementary material for: Classifier Language Models: Unifying Sparse Finetuning and Adaptive Tokenization for Specialized Classification Tasks
Source: arXiv:2508.08635 source file (2025-08-12)
Supplement: Supplementary file 4 [file other_attrs.tex]

\section{Evaluating on Other Attributes}
\label{appendix:other_attrs}

\begin{table*}[!htbp]
\centering
\tiny
\caption{Achieved delta for toxicity and formality across all approaches for different target deltas. The scores are averaged across three training runs (inference runs for GPT-3). We use a tolerance $\epsilon = 0.1$ for all of our approaches, as it empirically provided the best results in~\Cref{subsec:tolerance}. We find that our approaches (\textsc{Cev-LM ($\mathcal{N}$-only)} and \textsc{Cev-LM}) show significantly more control over all control conditions across nearly all target deltas.\vspace{-5pt}}
%\footnotesize
\noindent\setlength\tabcolsep{2.9pt}
\fontsize{5pt}{6pt}\selectfont
\resizebox{\textwidth}{!}{%
\begin{tabular}{@{}p{0.20\linewidth}@{\hspace{2pt}}
% K{\newfactor\linewidth}K{\newfactor\linewidth}K{\newfactor\linewidth}@{\hspace{5pt}}
% K{\newfactor\linewidth}K{\newfactor\linewidth}K{\newfactor\linewidth}@{\hspace{5pt}}
% % K{\newfactor\linewidth}K{\newfactor\linewidth}K{\newfactor\linewidth}@{\hspace{5pt}}
% K{\newfactor\linewidth}K{\newfactor\linewidth}K{\newfactor\linewidth}@{}} \\
ccc@{\hspace{5pt}}ccc@{\hspace{5pt}}ccc@{}}
\toprule
{\textbf{Metric}} & \multicolumn{3}{c}{\textbf{Toxicity}}  & \multicolumn{3}{c}{\textbf{Formality}} & \multicolumn{1}{c}{\textbf{\% Err}}\\
\cmidrule{2-4} \cmidrule(lr){5-7} \cmidrule{8-8}
%\midrule
{\textbf{Target Delta}} & \textbf{0.1} & \textbf{0.5} & \textbf{0.9} & \textbf{0.1} & \textbf{0.5} & \textbf{0.9}& - \\

\midrule
% Metric        &       & Toxicity &       &       & Formality &       & \multicolumn{1}{c}{% Err} \\
% Target Delta  & 0.1   & 0.5      & 0.9   & 0.1   & 0.5    & 0.9   & \multicolumn{1}{c}{-}     \\ \hline
% GPT-3         & 0.017 & 0.083    & 0.360 & 0.279 & 0.309  & 0.370 & 83.74                     \\
% MuCoCO        & 0.014 & 0.041    & 0.063 & 0.234 & 0.148  & 0.155 & 92.99                     \\
% SSD-LM        & 0.011 & 0.218    & 0.342 & 0.008 & 0.376  & 0.650 & 58.66                     \\
% Prefix Tuning & 0.188 & 0.397    & 0.978 & 0.273 & 0.339  & 0.941 & 54.50                     \\ \hline
% CEV-LM        & 0.075 & 0.325    & 0.709 & 0.162 & 0.427  & 0.810 & 27.97                    
\textbf{GPT-3}~\cite{brown2020language}      & 0.017 & 0.083    & 0.360 & 0.279 & 0.309  & 0.370 & 83.74 \\
\textbf{MuCoCO}~\cite{kumar2021controlled}   & 0.014 & 0.041    & 0.063 & 0.234 & 0.148  & 0.155 & 92.99 \\
\textbf{SSD-LM}~\cite{han2022ssd}            & 0.011 & 0.218    & 0.342 & 0.008 & 0.376  & 0.650 & 58.66  \\
\textbf{Prefix Tuning}~\cite{li2021prefix}   & 0.188 & \textbf{0.397}    & 0.978 & 0.273 & 0.339  & \textbf{0.941} & 54.50 \\
\midrule[0pt]
\textbf{\textsc{Cev-LM} (Ours)}                     & \textbf{0.075} & 0.325    & \textbf{0.709} & \textbf{0.162} & \textbf{0.427}  & 0.810 & \textbf{27.97}\\

\bottomrule
\end{tabular}}
% \vspace{-10pt}
\label{tab:other_attr_error}
\end{table*}

\begin{table*}[h]
\centering
\tiny
\caption{BLEU and BERT (F1) Scores for speed, volume, and circuitousness across all approaches for different target deltas. The scores are averaged across three training runs (inference runs for GPT-3). We use a tolerance $\epsilon = 0.1$ for all of our approaches, as it empirically provided the best results in~\Cref{subsec:tolerance}.\vspace{-5pt}}
%\footnotesize
\noindent\setlength\tabcolsep{2.9pt}
\fontsize{4pt}{4pt}\selectfont
\resizebox{\textwidth}{!}{%
\begin{tabular}{@{}p{0.20\linewidth}@{\hspace{2pt}}
% K{\newfactor\linewidth}K{\newfactor\linewidth}K{\newfactor\linewidth}@{\hspace{5pt}}
% K{\newfactor\linewidth}K{\newfactor\linewidth}K{\newfactor\linewidth}@{\hspace{5pt}}
% % K{\newfactor\linewidth}K{\newfactor\linewidth}K{\newfactor\linewidth}@{\hspace{5pt}}
% K{\newfactor\linewidth}K{\newfactor\linewidth}K{\newfactor\linewidth}@{}} \\
ccc@{\hspace{5pt}}ccc@{\hspace{5pt}}ccc@{}}
\toprule
\textbf{Metric} & \multicolumn{3}{c}{\textbf{Toxicity}}  & \multicolumn{3}{c}{\textbf{Formality}}\\
\cmidrule{2-4} \cmidrule(lr){5-7}
%\midrule
{\textbf{Target Delta}} & \textbf{0.1} & \textbf{0.5} & \textbf{0.9} & \textbf{0.1} & \textbf{0.5} & \textbf{0.9} \\

\midrule
\multicolumn{7}{c}{\textsc{\textbf{BERTScore} - Benchmark Approaches}} \\
\midrule[0pt]

\textbf{GPT-3}~\cite{brown2020language}       & 0.857 & 0.869    & 0.866 & 0.851 & 0.851  & 0.862  \\
\textbf{MuCoCO}~\cite{kumar2021controlled}    & 0.763 & 0.771    & 0.774 & 0.763 & 0.759  & 0.760  \\
\textbf{SSD-LM}~\cite{han2022ssd}             & 0.769 & 0.767    & 0.769 & 0.763 & 0.760  & 0.747 \\
\textbf{Prefix Tuning}~\cite{li2021prefix}    & 0.833 & 0.827    & 0.823 & 0.843 & 0.836  & 0.834  \\ 

\midrule[0pt]
\multicolumn{7}{c}{\textsc{\textbf{BERTScore} - Our Approaches}} \\
\midrule[0pt]

\textbf{\textsc{Cev-LM}}                      & 0.848 & 0.827    & 0.837 & 0.842 & 0.842  & 0.845   \\

\midrule
\multicolumn{7}{c}{\textsc{\textbf{BLEU} - Benchmark Approaches}} \\
\midrule[0pt]

\textbf{GPT-3}~\cite{brown2020language}       & 0.231 & 0.250    & 0.291 & 0.219 & 0.273     & 0.269 \\
\textbf{MuCoCO}~\cite{kumar2021controlled}    & 0.305 & 0.268    & 0.293 & 0.257 & 0.276     & 0.219 \\
\textbf{SSD-LM}~\cite{han2022ssd}             & 0.294 & 0.343    & 0.346 & 0.314 & 0.325     & 0.326   \\
\textbf{Prefix Tuning}~\cite{li2021prefix}    & 0.246 & 0.269    & 0.275 & 0.231 & 0.217     & 0.194 \\

\midrule[0pt]
\multicolumn{7}{c}{\textsc{\textbf{BLEU} - Our Approaches}} \\
\midrule[0pt]

\textbf{\textsc{Cev-LM}}                      & 0.320 & 0.316    & 0.295 & 0.342 & 0.334     & 0.265 \\

\bottomrule
\end{tabular}}
\label{tab:other_bleu_bert}
% \vspace{-10pt}
\end{table*}

% \begin{table}[]
% \begin{tabular}{lcccccc}
% \hline
% BERTScore     &       & Toxicity &       &       & Formality &        \\
% Target Delta  & 0.1   & 0.5      & 0.9   & 0.1   & 0.5    & 0.9    \\ \hline
% GPT-3         & 85.65 & 86.89    & 86.58 & 85.08 & 85.12  & 86.20  \\
% MuCoCO        & 76.31 & 77.08    & 77.41 & 76.31 & 75.92  & 76.01  \\
% SSD-LM        & 76.86 & 76.66    & 76.87 & 76.27 & 75.96  & 0.7472 \\
% Prefix Tuning & 83.21 & 82.73    & 82.27 & 84.34 & 83.60  & 83.39  \\ \hline
% CEV-LM        & 84.81 & 82.70    & 83.69 & 84.18 & 84.19  & 84.47 
% \end{tabular}
% \end{table}

% \begin{table}[]
% \begin{tabular}{lcccccc}
% \hline
% BLEU          &       & Toxicity &       &       & Formality &       \\
% Target Delta  & 0.1   & 0.5      & 0.9   & 0.1   & 0.5       & 0.9   \\ \hline
% GPT-3         & 0.231 & 0.250    & 0.291 & 0.219 & 0.273     & 0.269 \\
% MuCoCO        & 0.305 & 0.268    & 0.293 & 0.257 & 0.276     & 0.219 \\
% SSD-LM        & 0.294 & 0.343    & 0.346 & 0.314 & 0.325     & 0.326 \\
% Prefix Tuning & 0.246 & 0.269    & 0.275 & 0.231 & 0.217     & 0.194 \\ \hline
% CEV-LM        & 0.320 & 0.316    & 0.295 & 0.342 & 0.334     & 0.265
% \end{tabular}
% \end{table}
